# Supplementary material for: A new and practical formulation for overlaps of Bogoliubov vacua
Source: arXiv:2010.08459 ancillary file (2021-03-30)
Supplement: Supplementary file 1 [file sup6.pdf]

# Supplementary material for: A new and practical formulation for overlaps of Bogoliubov vacua

B. G. Carlsson and J. Rotureau
*Mathematical Physics, Lund University, S-221 00 Lund, Sweden*

### A. Even system

Let us consider two normalized HFB vacua $|\Phi\rangle$ and $|\Phi'\rangle$ containing an even number of particles. Each vacuum is expressed as a product of quasiparticles:

$$|\Phi\rangle = \frac{detC}{\prod_i v_i}\beta_0\ldots\beta_{N-1}|0\rangle \tag{1}$$

$$|\Phi'\rangle = \frac{detC'}{\prod_{i'} v'_i}\beta'_0\ldots\beta'_{N-1}|0\rangle. \tag{2}$$

The quasiparticle operators $\{\beta_i\}$ and $\{\beta'_i\}$ are given in terms of the matrices of the Bogoliubov transformation $(U,V)$ and $(U',V')$, respectively. The overlap $\mathcal{O} \equiv \langle\Phi|\Phi'\rangle$ reads:

$$\mathcal{O} = \frac{(detC)^* detC'}{\prod_{i,i'} v_i v'_i}\langle 0|\beta^\dagger_{N-1}\ldots\beta^\dagger_0\beta'_0\ldots\beta'_{N-1}|0\rangle \tag{3}$$

$$= (-1)^{N/2}\frac{(detC)^* detC'}{\prod_{i,i'} v_i v'_i}\langle 0|\beta^\dagger_0\ldots\beta^\dagger_{N-1}\beta'_0\ldots\beta'_{N-1}|0\rangle, \tag{4}$$

where the phase factor $(-1)^{N/2}$ in Eq. 4 stems from the rearrangement of the quasiparticle operators $\{\beta_i\}$. The matrix element in Eq. 4 can be expressed as the Pfaffian of all possible contractions [1–3]:

$$\mathcal{O} = (-1)^{N/2}\frac{(detC)^* detC'}{\prod_{i,i'} v_i v'_i}\mathrm{pf}(S), \tag{5}$$

where $S$ is a skew matrix of dimension $2N \times 2N$ defined as $S_{ij} = \langle 0|\hat{z}_i\hat{z}_j|0\rangle$ for $i<j$, and $\hat{z}_i$ is a generic notation for the quasiparticle creation and annihilation operators in (4). From the definition of the matrices $(U,V)$ and $(U',V')$, one can express the upper triangle of the matrix $S$ as:

$$S_{i,j} = \langle 0|\beta^\dagger_i\beta^\dagger_j|0\rangle = \left[V^T U\right]_{i,j}, \qquad 0 \le i < j \le N-1 \tag{6}$$

$$S_{i,N+j} = \langle 0|\beta^\dagger_i\beta'_j|0\rangle = \left[V^T V'^*\right]_{i,j} \quad 0 \le i \le N-1, \quad 0 \le j \le N-1 \tag{7}$$

$$S_{N+i,N+j} = \langle 0|\beta'_i\beta'_j|0\rangle = \left[U'^\dagger V'^*\right]_{i,j}, \qquad 0 \le i < j \le N-1, \tag{8}$$

while the lower triangle follows from $S$ being skew symmetric.

Using the above expression for $S$, the overlap can now be written as:

$$\mathcal{O} = (-1)^{N/2}\frac{(detC)^* detC'}{\prod_{i,i'} v_i v'_i}\mathrm{pf}\begin{pmatrix} V^T U & V^T V'^* \\ -V'^\dagger V & U'^\dagger V'^* \end{pmatrix}, \tag{9}$$

which corresponds to the expression for the overlap in [3]. Utilizing the Bloch-Messiah decompositions $\left(U = D\bar{U}C, V = D^*\bar{V}C\right)$ and $\left(U' = D'\bar{U}'C', V' = D'^*\bar{V}'C'\right)$ for the Bogoliubov matrices associated with $|\Phi\rangle$ and $|\Phi'\rangle$, respectively, we rewrite (9) as:

$$\mathcal{O} = (-1)^{N/2}\frac{(detC)^* detC'}{\prod_{i,i'} v_i v'_{i'}}\mathrm{pf}\begin{pmatrix} -C^T\bar{V}\bar{U}C & -C^T\bar{V}D^\dagger D'\bar{V}'C'^* \\ C'^\dagger\bar{V}'D'^T D^*\bar{V}C & C'^\dagger\bar{U}'\bar{V}'C'^* \end{pmatrix}. \tag{10}$$

By factorizing the matrix argument of the Pfaffian in (10), we can write:

$$\mathcal{O} = (-1)^{N/2} \frac{(detC)^* detC'}{\prod_{i,i'} v_i v'_{i'}} \text{pf} \left[ \begin{pmatrix} C^T & 0 \\ 0 & C'^{\dagger} \end{pmatrix} \begin{pmatrix} -\bar{V}\bar{U} & -\bar{V}D^{\dagger}D'\bar{V}' \\ \bar{V}'D'^T D^* \bar{V} & \bar{U}'\bar{V}' \end{pmatrix} \begin{pmatrix} C & 0 \\ 0 & C'^* \end{pmatrix} \right]. \tag{11}$$

From the relation

$$\text{pf}(ABA^T) = det(A)\text{pf}(B), \tag{12}$$

we obtain:

$$\mathcal{O} = (-1)^{N/2} \frac{1}{\prod_{i,i'} v_i v'_{i'}} \text{pf} \begin{pmatrix} -\bar{V}\bar{U} & -\bar{V}D^{\dagger}D'\bar{V}' \\ \bar{V}'D'^T D^* \bar{V} & \bar{U}'\bar{V}' \end{pmatrix}. \tag{13}$$

We factorize the matrix argument in the Pfaffian of Eq. (13) and write:

$$\mathcal{O} = (-1)^{N/2} \frac{1}{\prod_{i,i'} v_i v'_{i'}} \text{pf} \left[ \begin{pmatrix} \bar{V} & 0 \\ 0 & \bar{V}' \end{pmatrix} \begin{pmatrix} \bar{U}\bar{V}^{-1} & D^{\dagger}D' \\ -D'^T D^* & -\bar{V}'^{-1}\bar{U}' \end{pmatrix} \begin{pmatrix} -\bar{V} & 0 \\ 0 & -\bar{V}' \end{pmatrix} \right]. \tag{14}$$

By introducing the diagonal matrices

$$\Lambda = \begin{pmatrix} \sqrt{v_0} & & & & \\ & \sqrt{v_0} & & & \\ & & \sqrt{v_1} & & \\ & & & \ddots & \\ & & & & \sqrt{v_{N/2-1}} \end{pmatrix} \quad \text{and} \quad \Lambda' = \begin{pmatrix} \sqrt{v'_0} & & & & \\ & \sqrt{v'_0} & & & \\ & & \sqrt{v'_1} & & \\ & & & \ddots & \\ & & & & \sqrt{v'_{N/2-1}} \end{pmatrix} \tag{15}$$

we can now write (14) as :

$$\mathcal{O} = (-1)^{N/2} \frac{1}{\prod_{i,i'} v_i v'_{i'}} \text{pf} \left[ \begin{pmatrix} \bar{V}\Lambda^{-1} & 0 \\ 0 & \bar{V}'\Lambda'^{-1} \end{pmatrix} \begin{pmatrix} \Lambda\bar{U}\bar{V}^{-1}\Lambda & \Lambda D^{\dagger}D'\Lambda' \\ -\Lambda'D'^T D^* \Lambda & -\Lambda'\bar{V}'^{-1}\bar{U}'\Lambda' \end{pmatrix} \begin{pmatrix} -\Lambda^{-1}\bar{V} & 0 \\ 0 & -\Lambda'^{-1}\bar{V}' \end{pmatrix} \right]. \tag{16}$$

Using once again Eq. (12) we obtain:

$$\mathcal{O} = (-1)^{N/2} \frac{1}{\prod_{i,i'} v_i v'_{i'}} det(\bar{V}\Lambda^{-1}) det(\bar{V}'\Lambda'^{-1}) \begin{pmatrix} \Lambda\bar{U}\bar{V}^{-1}\Lambda & \Lambda D^{\dagger}D'\Lambda' \\ -\Lambda'D'^T D^* \Lambda & -\Lambda'\bar{V}'^{-1}\bar{U}'\Lambda' \end{pmatrix} \tag{17}$$

$$= (-1)^{N/2} \text{pf} \begin{pmatrix} \Lambda\bar{U}\bar{V}^{-1}\Lambda & \Lambda D^{\dagger}D'\Lambda' \\ -\Lambda'D'^T D^* \Lambda & -\Lambda'\bar{V}'^{-1}\bar{U}'\Lambda' \end{pmatrix} \tag{18}$$

Finally, introducing the matrix

$$\sigma = \begin{pmatrix} 0 & 1 & 0 & 0 & 0 \\ -1 & 0 & 0 & 0 & 0 \\ 0 & 0 & 0 & 1 & 0 \\ 0 & 0 & -1 & 0 & 0 \\ 0 & 0 & 0 & 0 & \ddots \end{pmatrix}, \tag{19}$$

we can now write

$$\mathcal{O} = (-1)^{N/2} \text{pf} \begin{pmatrix} -\bar{U}\sigma & \Lambda D^{\dagger}D'\Lambda' \\ -\Lambda'D'^T D^* \Lambda & \sigma\bar{U}' \end{pmatrix}. \tag{20}$$

The matrix argument of the Pfaffian in Eq. (20) can be reduced by setting to zero the coefficients $v_i$ ($v'_{i'}$) for which $v_i \leq \eta$ ($v'_i \leq \eta$), with $\eta$ a given parameter. Accordingly, the values of $u_i$ and $u'_i$ for the corresponding orbitals are set to one. In order to derive the expression for the overlap in this context, we will proceed in two steps. First, we set to zero the values of $v'_i$ which fulfills the criteria $v'_i \leq \eta$. Let us denote $n'$ the number of $v'_i > \eta$ and $\Delta' = N - n'$ the number of remaining $v'_i$, which are set to zero. In that case, the Pfaffian in Eq. (20) can be written as

$$\mathrm{pf}\begin{pmatrix} [-\bar{U}\sigma]_{N\times N} & [\Lambda D^\dagger D'\Lambda']_{N\times n'} & [0]_{N\times\Delta'} \\ -[\Lambda' D'^T D^*\Lambda]_{n'\times N} & [\sigma\bar{U}']_{n'\times n'} & [0]_{n'\times\Delta'} \\ [0]_{\Delta'\times N} & [0]_{\Delta'\times n'} & [\sigma]_{\Delta'\times\Delta'} \end{pmatrix}. \tag{21}$$

where the subscript attached to each block indicates their dimension. For instance, $[\Lambda D^\dagger D'\Lambda']_{N\times n'}$ is the matrix obtained by keeping only the first $N$ rows and $n'$ columns of matrix $\Lambda D^\dagger D'\Lambda'$. From the following relation fulfilled by the Pfaffian of a block matrix,

$$\mathrm{pf}\begin{pmatrix} A & 0 \\ 0 & B \end{pmatrix} = \mathrm{pf}(A)\mathrm{pf}(B), \tag{22}$$

we can write (21) as :

$$\mathrm{pf}\begin{pmatrix} [-\bar{U}\sigma]_{N\times N} & [\Lambda D^\dagger D'\Lambda']_{N\times n'} \\ -[\Lambda' D'^T D^*\Lambda]_{n'\times N} & [\sigma\bar{U}']_{n'\times n'} \end{pmatrix} \mathrm{pf}([\sigma]_{\Delta'\times\Delta'}) = \mathrm{pf}\begin{pmatrix} [-\bar{U}\sigma]_{N\times N} & [\Lambda D^\dagger D'\Lambda']_{N\times n'} \\ -[\Lambda' D'^T D^*\Lambda]_{n'\times N} & [\sigma\bar{U}']_{n'\times n'} \end{pmatrix}. \tag{23}$$

In the second step, we set to zero the values of $v_i$ which fulfills the criteria $v_i \leq \eta$ and we denote $n$ the number of $v_i > \eta$ and $\Delta = N - n$ the number of remaining vanishing $v_i$. The Pfaffian on the right-hand side of Eq. (23) then becomes:

$$\mathrm{pf}\begin{pmatrix} [-\bar{U}\sigma]_{n\times n} & [0]_{n\times\Delta} & [\Lambda D^\dagger D'\Lambda']_{n\times n'} \\ [0]_{\Delta\times n} & [-\sigma]_{\Delta\times\Delta} & [0]_{\Delta\times n'} \\ -[\Lambda' D'^T D^*\Lambda]_{n'\times n} & [0]_{n'\times\Delta} & [\sigma\bar{U}']_{n'\times n'} \end{pmatrix}. \tag{24}$$

By repeatedly using that interchange of two different rows and corresponding columns changes the sign of the Pfaffian, we can write the matrix in (24) as a block matrix and from Eq. 12 and Eq. 22, the Pfaffian (24) can be written as:

$$\mathrm{pf}\begin{pmatrix} [-\bar{U}\sigma]_{n\times n} & [\Lambda D^\dagger D'\Lambda']_{n\times n'} \\ -[\Lambda' D'^T D^*\Lambda]_{n'\times n} & [\sigma\bar{U}']_{n'\times n'} \end{pmatrix} \mathrm{pf}([-\sigma]_{\Delta\times\Delta}) \tag{25}$$

$$= \mathrm{pf}\begin{pmatrix} [-\bar{U}\sigma]_{n\times n} & [\Lambda D^\dagger D'\Lambda']_{n\times n'} \\ -[\Lambda' D'^T D^*\Lambda]_{n'\times n} & [\sigma\bar{U}']_{n'\times n'} \end{pmatrix} (-1)^{\Delta/2}. \tag{26}$$

Finally, from Eq. (20) and Eq. (26), the overlap in the truncated space can be written:

$$(-1)^{n/2}\mathrm{pf}\begin{pmatrix} [-\bar{U}\sigma]_{n\times n} & [\Lambda D^\dagger D'\Lambda']_{n\times n'} \\ -[\Lambda' D'^T D^*\Lambda]_{n'\times n} & [\sigma\bar{U}']_{n'\times n'} \end{pmatrix}. \tag{27}$$

### B. Odd system

We now consider the overlap between two states having odd particle numbers. Both states are constructed by acting with one quasi-particle creation operator on each even vacuum that is, $\beta_a^\dagger|\Phi\rangle$ and $\beta_{a'}^{'\dagger}|\Phi'\rangle$. The overlap is then obtained as:

$$\mathcal{O} = (-1)^{N/2}\frac{(detC)^* detC'}{\prod_{i,i'} v_i v'_{i'}} \langle 0|\beta_0^\dagger \dots \beta_{N-1}^\dagger \beta_a \beta_{a'}^{'\dagger} \beta_0^{'} \dots \beta_{N-1}^{'}|0\rangle. \tag{28}$$

As previously for the even case, we express the overlap with the Pfaffian of all possible contractions

$$\mathcal{O} = (-1)^{N/2}\frac{(detC)^* detC'}{\prod_{i,i'} v_i v'_{i'}} \mathrm{pf}(S) \tag{29}$$

where the matrix $S$ can be divided in 8 different blocks. From the definition of the matrices $(U, V)$ and $(U', V')$, one can express the upper triangle of the matrix $S$ as:

$$S_{i,j} = \langle 0|\beta_i^\dagger \beta_j^\dagger|0\rangle = \left[V^T U\right]_{i,j}, \qquad 0 \le i < j \le N-1 \tag{30}$$

$$S_{i,N} = \langle 0|\beta_i^\dagger \beta_a|0\rangle = \left[V^T V^*\right]_{i,a} \tag{31}$$

$$S_{i,N+1} = \langle 0|\beta_i^\dagger \beta_{a'}^{'\dagger}|0\rangle = \left[V^T U'\right]_{i,a'} \tag{32}$$

$$S_{i,N+2+j} = \langle 0|\beta_i^\dagger \beta_j^{'}|0\rangle = \left[V^T V'^*\right]_{i,j} \tag{33}$$

$$S_{N,N+1} = \langle 0|\beta_a \beta_{a'}^{'\dagger}|0\rangle = \left[U^\dagger U'\right]_{a,a'} \tag{34}$$

$$S_{N,N+2+j} = \langle 0|\beta_a \beta_j^{'}|0\rangle = \left[U^\dagger V'^*\right]_{a,j} \tag{35}$$

$$S_{N+1,N+2+j} = \langle 0|\beta_{a'}^{'\dagger} \beta_j^{'}|0\rangle = \left[V'^T V'^*\right]_{a',j} \tag{36}$$

$$S_{N+2+i,N+2+j} = \langle 0|\beta_i^{'} \beta_j^{'}|0\rangle = \left[U'^\dagger V'^*\right]_{i,j}, \quad 0 \le i < j \le N-1, \tag{37}$$

where if not specified $0 \le i \le N-1$ and $0 \le j \le N-1$. We use $\mathbf{U}^{(a)}$ and $\mathbf{V}^{(a)}$ to denote column vectors $a$ of the $U$ and $V$ matrices (with analogous notation for the matrices of the ket).

The matrix $S$ then reads:

$$S = \begin{pmatrix} V^T U & V^T \mathbf{V}^{(a)*} & V^T \mathbf{U}'^{(a')} & V^T V'^* \\ & 0 & \mathbf{U}^{(a)\dagger}\mathbf{U}'^{(a')} & \mathbf{U}^{(a)\dagger} V'^* \\ & & 0 & \mathbf{V}'^{(a')T} V'^* \\ & & & U'^\dagger V'^* \end{pmatrix}. \tag{38}$$

Since the matrix is skew symmetric, only the upper triangle is written out. Using the Bloch-Messiah decompositions of $(U, V)$ and $(U', V')$, we can write $S$ as:

$$S = \begin{pmatrix} -C^T \bar{V}\bar{U} C & -C^T \bar{V} D^\dagger \mathbf{V}^{(a)*} & -C^T \bar{V} D^\dagger \mathbf{U}'^{(a')} & -C^T \bar{V} D^\dagger D' \bar{V}' C'^* \\ & 0 & \mathbf{U}^{(a)\dagger}\mathbf{U}'^{(a')} & \mathbf{U}^{(a)\dagger} D' \bar{V}' C'^* \\ & & 0 & \mathbf{V}'^{(a')T} D' \bar{V}' C'^* \\ & & & C'^\dagger \bar{U}' \bar{V}' C'^* \end{pmatrix}. \tag{39}$$

$S$ can be factorized as:

$$S = \begin{pmatrix} C^T & 0 & 0 & 0 \\ 0 & 1 & 0 & 0 \\ 0 & 0 & 1 & 0 \\ 0 & 0 & 0 & C'^\dagger \end{pmatrix} \begin{pmatrix} -\bar{V}\bar{U} & -\bar{V} D^\dagger \mathbf{V}^{(a)*} & -\bar{V} D^\dagger \mathbf{U}'^{(a')} & -\bar{V} D^\dagger D' \bar{V}' \\ & 0 & \mathbf{U}^{(a)\dagger}\mathbf{U}'^{(a')} & \mathbf{U}^{(a)\dagger} D' \bar{V}' \\ & & 0 & \mathbf{V}'^{(a')T} D' \bar{V}' \\ & & & \bar{U}' \bar{V}' \end{pmatrix} \begin{pmatrix} C & 0 & 0 & 0 \\ 0 & 1 & 0 & 0 \\ 0 & 0 & 1 & 0 \\ 0 & 0 & 0 & C'^* \end{pmatrix}. \tag{40}$$

Using the relation Eq. (12) and the above factorized form of $S$, we can write the overlap (29) as:

$$\mathcal{O} = (-1)^{N/2} \frac{1}{\prod_{i,i'} v_i v'_{i'}} \mathrm{pf} \begin{pmatrix} -\bar{V}\bar{U} & -\bar{V} D^\dagger \mathbf{V}^{(a)*} & -\bar{V} D^\dagger \mathbf{U}'^{(a')} & -\bar{V} D^\dagger D' \bar{V}' \\ & 0 & \mathbf{U}^{(a)\dagger}\mathbf{U}'^{(a')} & \mathbf{U}^{(a)\dagger} D' \bar{V}' \\ & & 0 & \mathbf{V}'^{(a')T} D' \bar{V}' \\ & & & \bar{U}' \bar{V}' \end{pmatrix}. \tag{41}$$

We then factorize once again the matrix argument of the Pfaffian in Eq (41) and obtain:

$$\mathcal{O} = (-1)^{N/2} \frac{1}{\prod_{i,i'} v_i v'_{i'}} \mathrm{pf} \left[ \begin{pmatrix} -\bar{V} & 0 & 0 & 0 \\ & 1 & 0 & 0 \\ & & 1 & 0 \\ & & & -\bar{V}' \end{pmatrix} \begin{pmatrix} \bar{U}\bar{V}^{-1} & \bar{V} D^\dagger \mathbf{V}^{(a)*} & D^\dagger \mathbf{U}'^{(a')} & D^\dagger D' \\ & 0 & \mathbf{U}^{(a)\dagger}\mathbf{U}'^{(a')} & \mathbf{U}^{(a)\dagger} D' \\ & & 0 & \mathbf{V}'^{(a')T} D' \\ & & & -\bar{V}'^{-1} \bar{U}' \end{pmatrix} \begin{pmatrix} \bar{V} & 0 & 0 & 0 \\ & 1 & 0 & 0 \\ & & 1 & 0 \\ & & & \bar{V}' \end{pmatrix} \right]. \tag{42}$$

Introducing the diagonal matrix $\Lambda$ and $\Lambda'$ (15), we can now write:

$$\mathcal{O} = \frac{(-1)^{N/2}}{\prod_{i,i'} v_i v'_{i'}} \mathrm{pf}\left[\begin{pmatrix} -\bar{V}\Lambda^{-1} & 0 & 0 & 0 \\ & 1 & 0 & 0 \\ & & 1 & 0 \\ & & & -\bar{V}'\Lambda'^{-1} \end{pmatrix}\begin{pmatrix} \Lambda\bar{U}\bar{V}^{-1}\Lambda & \Lambda D^\dagger \mathbf{V}^{(a)*} & \Lambda D^\dagger \mathbf{U}'^{(a')} & \Lambda D^\dagger D'\Lambda' \\ & 0 & \mathbf{U}^{(a)\dagger}\mathbf{U}'^{(a')} & \mathbf{U}^{(a)\dagger} D'\Lambda' \\ & & 0 & \mathbf{V}'^{(a')T} D'\Lambda' \\ & & & -\Lambda'\bar{V}'^{-1}\bar{U}'\Lambda' \end{pmatrix}\begin{pmatrix} \Lambda^{-1}\bar{V} & 0 & 0 & 0 \\ & 1 & 0 & 0 \\ & & 1 & 0 \\ & & & \Lambda'^{-1}\bar{V}' \end{pmatrix}\right]. \tag{43}$$

Using once again Eq. (12), we obtain:

$$\mathcal{O} = (-1)^{N/2}\mathrm{pf}\begin{pmatrix} -\bar{U}\sigma & \Lambda D^\dagger \mathbf{V}^{(a)*} & \Lambda D^\dagger \mathbf{U}'^{(a')} & \Lambda D^\dagger D'\Lambda' \\ & 0 & \mathbf{U}^{(a)\dagger}\mathbf{U}'^{(a')} & \mathbf{U}^{(a)\dagger} D'\Lambda' \\ & & 0 & \mathbf{V}'^{(a')T} D'\Lambda' \\ & & & \sigma\bar{U}' \end{pmatrix}. \tag{44}$$

The expression can be rearranged as:

$$\mathcal{O} = (-1)^{N/2}\mathrm{pf}\begin{pmatrix} -\bar{U}\sigma & \Lambda D^\dagger D'\Lambda' & \Lambda D^\dagger \mathbf{V}^{(a)*} & \Lambda D^\dagger \mathbf{U}'^{(a')} \\ & \sigma\bar{U}' & -\Lambda' D'^T \mathbf{U}^{(a)*} & -\Lambda' D'^T \mathbf{V}'^{(a')} \\ & & 0 & \mathbf{U}^{(a)\dagger}\mathbf{U}'^{(a')} \\ & & & 0 \end{pmatrix} = (-1)^{N/2}\mathrm{pf}\begin{pmatrix} \mathcal{A} & \mathcal{B} \\ -\mathcal{B}^T & \mathcal{C} \end{pmatrix} \tag{45}$$

In this form, one matrix is related to the even part of the system

$$\mathcal{A} = \begin{pmatrix} -\bar{U}\sigma & \Lambda D^\dagger D'\Lambda' \\ -\Lambda' D'^T D^*\Lambda & \sigma\bar{U}' \end{pmatrix}, \tag{46}$$

one related to the connection between the even and the odd part

$$\mathcal{B} = \begin{pmatrix} \Lambda D^\dagger & 0 \\ 0 & -\Lambda' D'^T \end{pmatrix}\begin{pmatrix} \mathbf{V}^{(a)*} & \mathbf{U}'^{(a')} \\ \mathbf{U}^{(a)*} & \mathbf{V}'^{(a')} \end{pmatrix}, \tag{47}$$

and one matrix related to the odd particles

$$\mathcal{C} = \begin{pmatrix} 0 & \mathbf{U}^{(a)\dagger}\mathbf{U}'^{(a')} \\ -\mathbf{U}^{(a)\dagger}\mathbf{U}'^{(a')} & 0 \end{pmatrix}. \tag{48}$$

As in the even case, truncations of the matrix argument of the Pfaffian can be performed by fixing to zero the values $v_i \leq \eta$ ($v'_{i'} \leq \eta$) associated with the even vacua $|\Phi\rangle$ and $|\Phi'\rangle$. The derivation of the overlap is similar to the case of the overlap for an even system but becomes more tedious due the addition of the quasiparticle associated with the odd system. Using the same notation as in the even case, the truncated expression for the overlap (45) reads:

$$\mathcal{O} = (-1)^{n/2}\mathrm{pf}\begin{pmatrix} -[\bar{U}\sigma]_{n\times n} & [\Lambda D^\dagger D'\Lambda']_{n\times n'} & [\Lambda D^\dagger \mathbf{V}^{(a)*}]_{n\times 1} & [\Lambda D^\dagger \mathbf{U}'^{(a')}]_{n\times 1} \\ & [\sigma\bar{U}']_{n'\times n'} & -[\Lambda' D'^T \mathbf{U}^{(a)*}]_{n'\times 1} & -[\Lambda' D'^T \mathbf{V}'^{(a')}]_{n'\times 1} \\ & & 0 & [\mathbf{U}^{(a)\dagger}\mathbf{U}'^{(a')}]_{1\times 1} \\ & & & 0 \end{pmatrix}. \tag{49}$$

[1] E. H. Lieb, Journal of Combinatorial Theory **5**, 313 (1968).
[2] E. R. Caianiello, *Combinatorics and renormalization in quantum field theory* (W. A. Benjamin Reading, Mass, 1973).
[3] G. F. Bertsch and L. M. Robledo, Phys. Rev. Lett. **108**, 042505 (2012).
